# Supplementary material for: Quantum fluxes at the inner horizon of a spinning black hole
Source: arXiv:2203.08502 ancillary file (2022-12-14)
Supplement: Supplementary file 1 [file sup35.pdf]

# Supplemental Material for:

# Quantum fluxes at the inner horizon of a spinning black hole

Noa Zilberman, Marc Casals, Amos Ori and Adrian Ottewill

This document is the Supplemental Material for the manuscript "Quantum fluxes at the inner horizon of a spinning black hole", and is organized as follows: Section 1 deals with the effective potential $V_{\omega lm}$; Section 2 consists of basic details regarding the numerical implementation of the flux computation; Section 3 presents results for the polar fluxes at $r$ values off the IH, computed via point splitting – focusing on their IH limit, and comparing them to the values obtained (in the main manuscript) directly at the IH via the state-subtraction method; Finally, Section 4 presents the behavior of the polar fluxes in the near-extremal domain.

## 1 The effective potential

The effective potential is

$$V_{\omega lm}(r) = \frac{K_{\omega m}^2(r) - \lambda_{lm}(a\omega)\,\Delta}{\left(r^2+a^2\right)^2} - G^2(r) - \frac{\Delta}{r^2+a^2}\frac{\mathrm{d}G(r)}{\mathrm{d}r} \tag{1}$$

where

$$K_{\omega m}(r) \equiv \left(r^2+a^2\right)\omega - am\,, \quad \lambda_{lm}(a\omega) \equiv E_{lm}(a\omega) - 2am\omega + a^2\omega^2 \tag{2}$$

($E_{lm}(a\omega)$ being the angular eigenvalue, see e.g. Eq. (2.16) in [1]) and

$$G(r) \equiv \frac{r\Delta}{\left(r^2+a^2\right)^2}\,. \tag{3}$$

Evidently, as mentioned in Eq. (4) in the main manuscript, $V_{\omega lm}$ goes to $\omega_{\pm}^2$ at $r \to r_{\pm}$. Furthermore, the next order of $V_{\omega lm}$ in these asymptotic domains goes like $\propto e^{\pm 2\kappa_{\pm} r_*}$. Thus, the potential is short-ranged. This justifies the free asymptotic forms given in Eqs. (5) and (6) in the main manuscript.

Note also that the potential is regular at $r = 0$, and in fact on the entire real axis.

# 2 The numerical setup

The computation of the fluxes at the IH follows the prescription presented in Eqs. (12), (13) and (7) in the main manuscript. The primary numerical effort required is the computation of the internal scattering parameters $A_{\omega lm}$ and $B_{\omega lm}$, as well as the reflection coefficient $\rho_{\omega lm}^{\mathrm{up}}$ defined in the BH exterior. The methods used for this computation are outlined in Subsec. 2.1. Subsequently, we need to implement the mode sum (i.e. to sum and integrate over the contributions of the individual modes). This task, which is more straightforward, is briefly described in Subsec. 2.2.

## 2.1 Computing the scattering parameters $A_{\omega lm}$, $B_{\omega lm}$ and $\rho_{\omega lm}^{\mathbf{up}}$

We used the so-called MST method (see [2] for a review) for calculating the scattering parameters $A_{\omega lm}$, $B_{\omega lm}$ and $\rho_{\omega lm}^{\mathrm{up}}$. Within the MST method, outer solutions of the radial equation (Eq. (3) in the main text) are expressed as infinite series of (ordinary and confluent) hypergeometric functions, with expansion coefficients satisfying a three-term recurrence relation and involving a parameter (the so-called renormalized angular momentum) which is determined so that the series converge. The various series then converge in different radial intervals, none of which includes the whole outer scattering regime (namely, from $r = r_+$ to $r \to \infty$). By appropriately matching the series in a region of overlap and then taking their $r \to r_+$ and $r \to \infty$ limits, analytic expressions for the outer scattering parameters as infinite sums involving the expansion coefficients and the renormalized angular momentum parameter can be read off.

An expression for the outer scattering parameter $\rho_{\omega lm}^{\mathrm{up}}$ of the upgoing radial solution (defined via Eq. (3.3) in [1]) can be readily obtained, by using the Wronskian relations (see Eq. (3.33) in

[1]), in terms of the scattering parameters of the ingoing radial solution (defined via Eq. (3.2) in [1]). In their turn, MST expressions for these scattering parameters of the ingoing solution are given in Eqs. (167)-(169) in [2] and are implemented in the Black Hole Perturbation Toolkit [3]. This allowed us to obtain $\rho^{\rm up}_{\omega lm}$ to any desired precision.

On the other hand, to the best of our knowledge, there are no available MST expressions for the *inner* scattering parameters $A_{\omega lm}$ and $B_{\omega lm}$ (see Eq. (6) in the main text). Taking the aforementioned MST series for the ingoing radial solution outside the BH and adapting it to form a series for $\psi^{\rm int}_{\omega lm}$ valid inside the BH, and then taking the limit of this series to $r = r_-$ and equating it to the boundary condition there (Eq. (6) in the main text), we obtained MST-based expressions for $A_{\omega lm}$ and $B_{\omega lm}$. We implemented and evaluated these expressions in Wolfram Mathematica.

We independently derived expressions for $\psi^{\rm int}_{\omega lm}$, $A_{\omega lm}$ and $B_{\omega lm}$ in terms of the confluent Heun function of argument $(r-r_-)/(r_+-r_-)$ and $(r_+-r)/(r_+-r_-)$ and their Wronskians and numerically validated our alternate expressions against each other to high precision.

## 2.2 Implementing the mode-sum

We have computed $A_{\omega lm}$, $B_{\omega lm}$ and $\rho^{\rm up}_{\omega lm}$ (as described in the previous subsection) as well as the spheroidal wavefunction $S^{\omega}_{lm}(\theta)$ for the required set of modes. This set generally takes the form $0 \le l \le l_{\max}$, $-l \le m \le l$, and the frequency range $0 < \omega \le \omega_{\max}$ with some stepsize $d\omega$; hence it is characterized by the three parameters $l_{\max}$, $\omega_{\max}$, and $d\omega$. For $\theta = 0$ we need only $m = 0$ (since $S^{\omega}_{l,m\neq 0}$ vanishes there), which means the polar flux computation requires much less modes (compared to the $\theta \neq 0$ case), making it significantly easier to implement.

At the pole, we computed the fluxes in a variety of spin values in the range $0.55 \le a/M \le 0.99999$. For $a/M \le 0.999$ we used $l_{\max} = 10$, $\omega_{\max} = 10/M$ and $d\omega = 0.005/M$. However, as we move deeper into the near-extremal domain, the required range in $\omega$ (as well as the required increment $d\omega$) typically scales down with the deviation from extremality. Thus, at $a/M > 0.999$ we used $\omega_{\max} = 1/M$ and $d\omega = 10^{-4}/M$ with $l_{\max} = 5$ (although we could have managed with much smaller $l_{\max}$, e.g. $l_{\max} = 2$).

For $a/M = 0.8$ we also computed the fluxes off the pole. As $\theta$ increases towards $\pi/2$, we

find that the convergence rate (in both $l$ and $\omega$) becomes significantly slower, which requires increasing $l_{\max}$ and $\omega_{\max}$. For $\theta = \pi/2$ (which is the hardest to compute) we used frequencies up to $\omega_{\max} = 30/M$ with $l_{\max} = 40$.

With all the ingredients (namely $\rho^{\mathrm{up}}_{\omega lm}$, $A_{\omega lm}$, $B_{\omega lm}$ and $S^{\omega}_{lm}(\theta)$) at hand, we now construct the integrands for $\langle T^{-}_{uu}\rangle^{U}_{\mathrm{ren}}$ and $\langle T^{-}_{vv}\rangle^{U}_{\mathrm{ren}}$ as given in Eqs. (12) and (13) (along with Eq. (7)) in the main manuscript. Then, having constructed the integrands, we perform the summation (over $l, m$) and integration (over $\omega$). In the first step we sum over $m$ for each given $\omega$ and $l$. We then find exponential decay both in $l$ (per given $\omega$) and in $\omega$ (per given $l$). Thus the convergence is uniform and we can freely choose the order of summation over $l$ and integration over $\omega$. We tried both orders, and they indeed produced the same results. The values of $\omega_{\max}$ and $l_{\max}$ are chosen such that we are always deep in the exponential decay regime.

Finally we point out that in all plots (both in the main manuscript and in the supplemental materials), the points displayed have an error small enough to not be visually discernible.

# 3 Point-splitting flux values at the IH limit

Independently of the work presented in this paper, we have also computed [4] the trace-reversed [1] flux components denoted $\left\langle \overline{T}_{vv}\right\rangle^{U}_{\mathrm{ren}}$ and $\left\langle \overline{T}_{uu}\right\rangle^{U}_{\mathrm{ren}}$ (again for a minimally-coupled massless scalar field in the Unruh state inside a Kerr BH) using the point-splitting method [5] – specifically with a splitting in the $t$ direction, i.e. via the so-called *t-splitting* variant [6, 7]). The goal of this section is to compare these point-splitting results to those obtained in the present work via the state-subtraction method.

The point-splitting method (and particularly its $t$-splitting variant) is technically much harder to apply than state-subtraction. (In particular, the number of modes required for its application inside a Kerr BH is typically larger by a few orders of magnitudes than the state-subtraction computation at the IH.) For this reason, so far we have computed the (trace-reversed) fluxes inside

[1] The traced reversed stress-energy tensor is defined by $\overline{T}_{\alpha\beta} \equiv T_{\alpha\beta} - (1/2) g_{\alpha\beta} T^{\mu}{}_{\mu}$. In Ref. [4] we chose to compute the trace-reversed fluxes, rather than the fluxes themselves, since the latter would also require knowledge of the trace, which complicates the analysis. As will be discussed below, the difference between the ordinary fluxes and their trace-revered counterpart disappears at the IH limit, which concerns us here.

Kerr via point splitting only at the pole (i.e. $\theta = 0$, which further reduces the required mode ranges to $m = 0$ alone), and only for two spin values, $a/M = 0.8$ and $a/M = 0.9$. Furthermore, we are unable to perform a point-splitting computation directly at the IH of Kerr [2]. Instead, in Ref. [4] we computed the (trace-reversed) fluxes along the polar axis of Kerr in a variety of $r$ values in between the EH and IH. Here we shall focus our attention on the $r$ values in the close vicinity of the IH. We shall deduce the ($t$-splitting) flux values at the IH by evaluating the $r \to r_-$ limit of these near-IH (trace-reversed) flux values. [To this end, we recall that at the IH itself the ordinary (i.e. non-trace-reversed) fluxes and the trace-reversed fluxes coincide, because $\overline{T}_{\alpha\beta} \equiv T_{\alpha\beta} - (1/2) g_{\alpha\beta} T^{\mu}{}_{\mu}$, and both $g_{uu}$ and $g_{vv}$ vanish (like $(r - r_-)^2$) as $r \to r_-$.] Then we shall compare these limiting ($t$-splitting) flux values to those obtained in the present paper using the state-subtraction method. We will focus on two $a/M$ values at the pole: $a/M = 0.8$, in which the IH fluxes are positive, and $a/M = 0.9$, in which they are negative.

Figure 1 displays our $t$-splitting results for $\left\langle \overline{T}_{uu} \right\rangle_{\text{ren}}^{U}$ and $\left\langle \overline{T}_{vv} \right\rangle_{\text{ren}}^{U}$ at $a/M = 0.8$ as functions of $\delta r \equiv (r - r_-)/M$, presented in the range $2 \times 10^{-5} \leq \delta r \leq 5 \times 10^{-3}$ (well inside the near-IH domain). The two horizontal dashed lines denote the corresponding flux values obtained at the IH via state subtraction, and the approach of the two colorful curves to these two horizontal lines is very clearly seen.

In fact, the extrapolation of the two data sets (i.e. for $\left\langle \overline{T}_{uu} \right\rangle_{\text{ren}}^{U}$ and $\left\langle \overline{T}_{vv} \right\rangle_{\text{ren}}^{U}$) to $r = r_-$ allows us to obtain both limiting flux quantities with four robust significant figures: $\langle T_{vv}^{-} \rangle_{\text{ren}}^{U} \approx 0.00003013\, \hbar M^{-4}$ and $\langle T_{uu}^{-} \rangle_{\text{ren}}^{U} \approx 0.00003232\, \hbar M^{-4}$. The corresponding values obtained by the state-subtraction method are $\langle T_{vv}^{-} \rangle_{\text{ren}}^{U} \approx 0.0000301345442\, \hbar M^{-4}$ and $\langle T_{uu}^{-} \rangle_{\text{ren}}^{U} \approx 0.0000323163918\, \hbar M^{-4}$ – in full agreement (within numerical uncertainty) with the aforementioned $t$-splitting results. This remarkable agreement between the results obtained via $t$-splitting and state-subtraction provides strong support to both renormalization methods.

Figure 2 is the $a/M = 0.9$ counterpart of Figure 1. Extrapolation of the $t$-splitting results to $r = r_-$ yields $\langle T_{vv}^{-} \rangle_{\text{ren}}^{U} \approx -2.324 \times 10^{-6}\, \hbar M^{-4}$ and $\langle T_{uu}^{-} \rangle_{\text{ren}}^{U} \approx -1.702 \times 10^{-6}\, \hbar M^{-4}$. The corresponding values obtained by the state-subtraction method are $\langle T_{vv}^{-} \rangle_{\text{ren}}^{U} \approx -2.32381785 \times 10^{-6}\, \hbar M^{-4}$ and

[2] In the analogous RN case we have been able to compute the fluxes directly at the IH using the $\theta$-splitting variant of point splitting, see [8]. In the Kerr case, however, $\theta$-splitting is inapplicable and we therefore use the $t$-splitting variant, whose direct application on the IH is not possible.

$\langle T^{-}_{uu}\rangle^{U}_{\rm ren} \approx -1.70204120 \times 10^{-6}\,\hbar M^{-4}$. This agreement provides yet another piece of support for our method (this time for an $a/M$ value for which negative IH fluxes are attained).

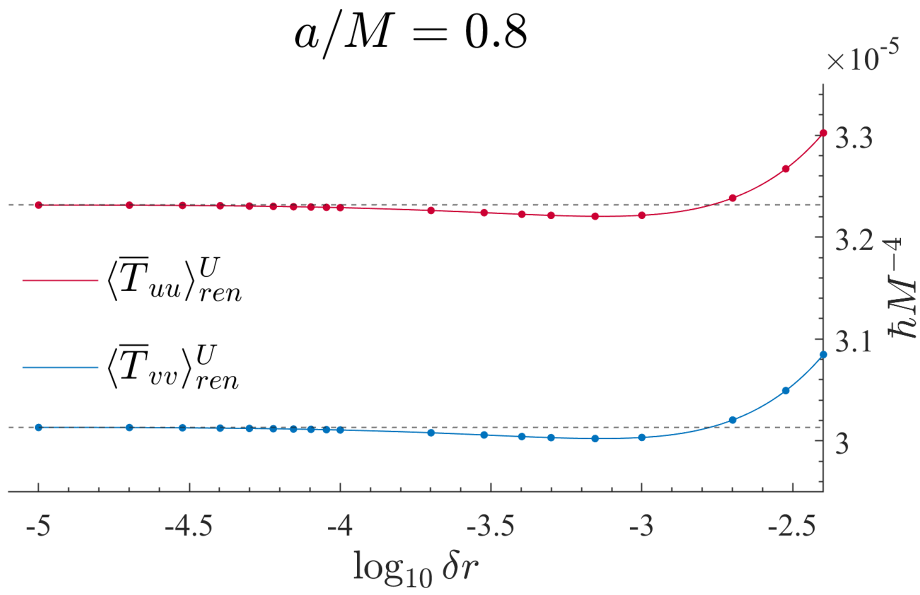


Figure 1: The polar $\langle \overline{T}_{vv}\rangle^{U}_{\rm ren}$ and $\langle \overline{T}_{uu}\rangle^{U}_{\rm ren}$ for $a/M = 0.8$ as functions of $\log_{10} \delta r$ at the IH vicinity. The dots denote values computed using $t$-splitting, and the lines connecting them are interpolations. The dashed horizontal lines denote the IH values, $\langle T^{-}_{vv}\rangle^{U}_{\rm ren}$ and $\langle T^{-}_{uu}\rangle^{U}_{\rm ren}$ correspondingly, computed in the state-subtraction method. The figure indeed demonstrates the consistency of the $r \to r_{-}$ limit (corresponding to going leftwards) with the value computed directly at the IH (via state-subtraction), as the colored lines approach the dashed horizontal ones.

## 4 The near-extremal domain

This section focuses on the behavior of the polar (i.e. $\theta = 0$) IH fluxes at the near-extremal domain.

Throughout this work we considered sub-extremal BHs (i.e. $a/M < 1$), but also pushed our calculations towards the extremal limit, reaching an $a/M$ value of 0.99999. As seen in Fig. 2 in the main manuscript, the polar IH fluxes $\langle T^{-}_{vv}\rangle^{U}_{\rm ren}$ and $\langle T^{-}_{uu}\rangle^{U}_{\rm ren}$ (as functions of $a/M$) decay as $a/M$ approaches the extremal limit of 1. This decay behavior towards extremality is also present in

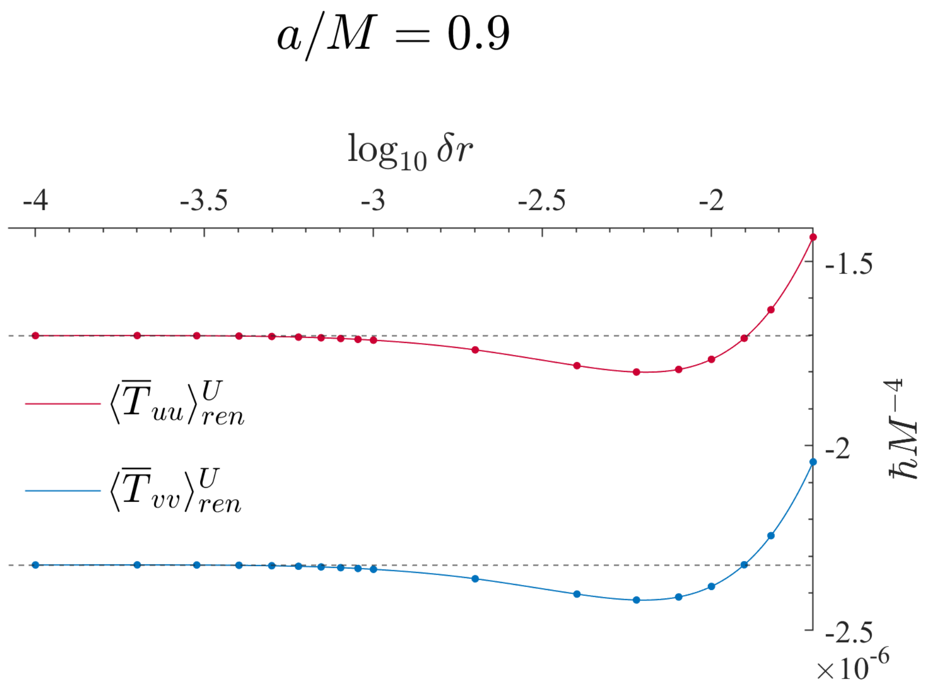


Figure 2: The same as in Figure 1, but for $a/M = 0.9$.

the analogous spherical charged case (see Ref. [8]). In Ref. [9] we focused on the near-extremal domain in the RN case, and investigated (both analytically and numerically) the behavior of the fluxes as a function of the parameter [3] $\Delta \equiv \sqrt{1-(Q/M)^2} \ll 1$. In particular, we found that $\langle T^{-}_{vv} \rangle^{U}_{\text{ren}}$ behaves as $\propto \Delta^4$ (with the prefactor calculated analytically), and that $\langle T^{-}_{uu} \rangle^{U}_{\text{ren}}$ behaves as $\propto \Delta^5$.

Similarly, in order to quantify near-extremality in Kerr, we define the small parameter $\epsilon \equiv \sqrt{1-(a/M)^2}$ (the spinning counterpart of $\Delta$ given above for the RN case). The near-extremal domain in Kerr is then characterized by $\epsilon \ll 1$.

Focusing on the near-extremal domain of our results (in Kerr), we investigated the behavior of the polar IH fluxes as a function of $\epsilon$ as the latter decreases, as described below. We found that, in analogy with the RN case, $\langle T^{-}_{vv} \rangle^{U}_{\text{ren}} \propto \epsilon^4$ and $\langle T^{-}_{uu} \rangle^{U}_{\text{ren}} \propto \epsilon^5$, both with negative coefficients (which we shall soon provide) [4].

---

[3] Do not confuse this $\Delta$ parameter (that was defined in Ref. [9] in the RN context) with $\Delta \equiv r^2 + a^2 - 2Mr$ used throughout the present paper.

[4] Note again that throughout this section, $\langle T^{-}_{vv} \rangle^{U}_{\text{ren}}$ and $\langle T^{-}_{uu} \rangle^{U}_{\text{ren}}$ refer to the $\theta = 0$ value of the IH fluxes.

It is also interesting to consider a third, related, quantity:

$$\mathcal{F} \equiv (r_-^2 + a^2) \left( \langle T_{uu}^- \rangle_{\rm ren}^U - \langle T_{vv}^- \rangle_{\rm ren}^U \right) \tag{4}$$

(where both the LHS and the RHS refer to the value at the pole), which actually coincides with the Hawking-radiation flux density per unit solid angle in the polar direction (owing to energy-momentum conservation – see Subsec. B2 in Ref. [1]). Then, combining $\langle T_{vv}^- \rangle_{\rm ren}^U \propto \epsilon^4$ and $\langle T_{uu}^- \rangle_{\rm ren}^U \propto \epsilon^5$ with Eq. (4), we find $\mathcal{F} \simeq -2M^2 \langle T_{vv}^- \rangle_{\rm ren}^U$ in the near-extremal domain (since to leading order in $\epsilon$ we have $r_- \simeq a \simeq M$).

As in the analogous RN case, we were able to analytically find the near-extremal leading order coefficient of $\langle T_{vv}^- \rangle_{\rm ren}^U$:

$$\langle T_{vv}^- \rangle_{\rm ren}^U \simeq -\frac{\hbar M^{-4}}{7680\pi^2}\,\epsilon^4 \tag{5}$$

(which turns out to be exactly 1/16 of the analogous RN result, given in Eq. (III.6) in Ref. [9]). Correspondingly, the Hawking radiation density per solid angle in the polar direction is

$$\mathcal{F} \simeq \frac{\hbar M^{-2}}{3840\pi^2}\,\epsilon^4 \tag{6}$$

(which is 1/8 of the corresponding quantity in RN: compare with Eq. (III.2) in Ref. [9], which should be divided by $4\pi$ to yield the Hawking radiation density per unit solid angle). We hope to present this analysis in a future paper.

For $\langle T_{uu}^- \rangle_{\rm ren}^U$ we numerically obtained the near-extremal leading order behavior:

$$\langle T_{uu}^- \rangle_{\rm ren}^U \approx -0.000105542\,\hbar M^{-4}\,\epsilon^5 \tag{7}$$

(compare with Eq. (III.4) in Ref. [9] for the analogous RN case). [5]

Fig. 3 displays the three quantities of interest (divided by their corresponding leading order powers of $\epsilon$) in the near-extremal domain, as a function of $\log_{10}\epsilon$. Extremality is reached at $\log_{10}\epsilon \to -\infty$, and the three plots indeed flatten leftwards to reach their leading order coefficients

[5] We also numerically computed the leading order near-extremal coefficients independently for $\langle T_{vv}^- \rangle_{\rm ren}^U$ and $\mathcal{F}$, and found an agreement of at least 5 robust figures with the analytical results given in Eqs. (5) and (6).

(found numerically for $\langle T^{-}_{uu}\rangle^{U}_{\rm ren}$ and analytically for the two others), represented by horizontal dashed lines. We choose to rescale $\mathcal{F}$ in the graph to have the same leading order behavior as that of $\langle T^{-}_{vv}\rangle^{U}_{\rm ren}$ (in suitable units), hence display $-(1/2)\mathcal{F} = (1/2)(r_-^2 + a^2)(\langle T^{-}_{vv}\rangle^{U}_{\rm ren} - \langle T^{-}_{uu}\rangle^{U}_{\rm ren})$ rather than $\mathcal{F}$. In addition, $\langle T^{-}_{uu}\rangle^{U}_{\rm ren}$ in the graph is multiplied by a factor of 1/3 just for convenience, to maintain the vertical scale of the plot.

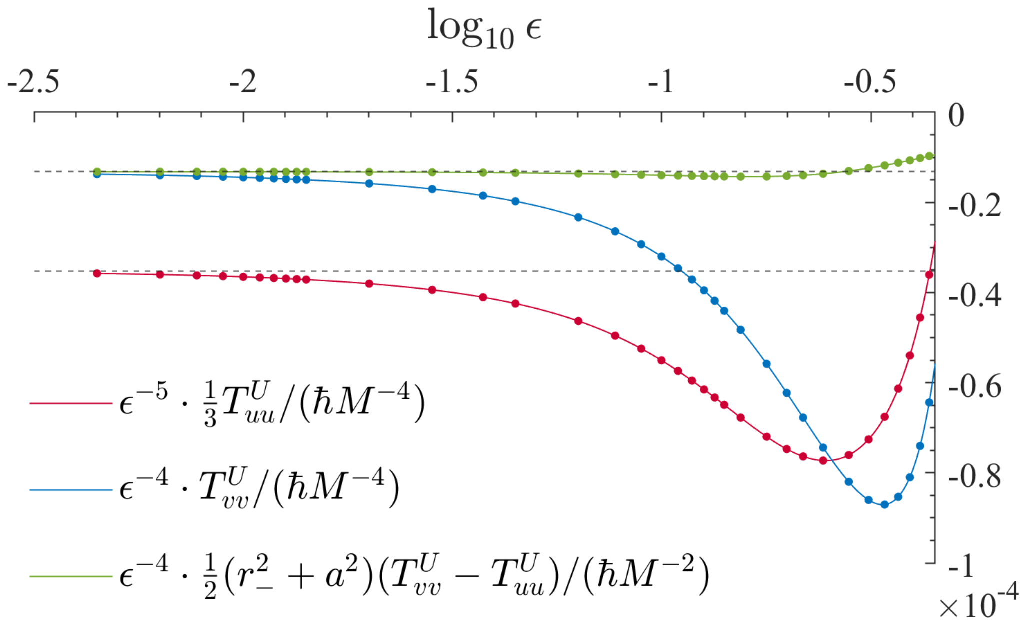


Figure 3: The polar IH quantities $\langle T^{-}_{vv}\rangle^{U}_{\rm ren}\,\epsilon^{-4}$, $(1/3)\,\langle T^{-}_{uu}\rangle^{U}_{\rm ren}\,\epsilon^{-5}$ and $(1/2)\left(r_-^2 + a^2\right)\left(\langle T^{-}_{vv}\rangle^{U}_{\rm ren} - \langle T^{-}_{uu}\rangle^{U}_{\rm ren}\right)\epsilon^{-4}$ (in suitable units) vs. $\log_{10}\epsilon$. The dashed horizontal lines correspond to the coefficients of the leading orders in $\epsilon$, see Eqs. (5) and (7). As expected, the two quantities $\langle T^{-}_{vv}\rangle^{U}_{\rm ren}\,/\,(\hbar M^{-4})$ and $(1/2)\left(r_-^2 + a^2\right)\left(\langle T^{-}_{vv}\rangle^{U}_{\rm ren} - \langle T^{-}_{uu}\rangle^{U}_{\rm ren}\right)/\,(\hbar M^{-2})$ share the same leading order coefficient.

# References


[1] N. Zilberman, M. Casals, A. Ori, and A. Ottewill, *Two-point function of a quantum scalar field in the interior region of a Kerr black hole*, arXiv:2203.07780 (submitted to Phys. Rev. D, temporary ID: es2022apr14-666).

[2] M. Sasaki and H. Tagoshi, *Analytic Black Hole Perturbation Approach to Gravitational Radiation*, Living Rev. Relativity **6**, 6 (2003).

[3] Black Hole Perturbation Toolkit, (bhptoolkit.org).

[4] N. Zilberman, M. Casals, A. Ori, and A. Ottewill, *in preperation.*

[5] S. M. Christensen, *Vacuum expectation value of the stress tensor in an arbitrary curved background: The covariant point separation method*, Phys. Rev. D. **14**, 2490 (1976).

[6] A. Levi, *Renormalized stress-energy tensor for stationary black holes*, Phys. Rev. D. **95**, 025007 (2017).

[7] A. Levi, E. Eilon, A. Ori and M. van de Meent, *Renormalized Stress-Energy Tensor of an Evaporating Spinning Black Hole*, Phys. Rev. Lett. **118**, 141102 (2017).

[8] N. Zilberman, A. Levi and A. Ori, *Quantum Fluxes at the Inner Horizon of a Spherical Charged Black Hole*, Phys. Rev. Lett. **124**, 171302 (2020).

[9] N. Zilberman and A. Ori, *Quantum fluxes at the inner horizon of a near-extremal spherical charged black bole*, Phys. Rev. D **104**, 024066 (2021).
